# Supplementary material for: Milky Way Accelerometry via Millisecond Pulsar Timing
Source: arXiv:2008.13052 source file (2021-04-15)
Supplement: Supplementary file 1 [file SM.pdf]

# Milky Way Accelerometry via Millisecond Pulsar Timing: Supplemental Material

David F. Phillips,[1,*] Aakash Ravi,[2,†] Reza Ebadi,[2,3] and Ronald L. Walsworth[2,3,4]

[1] *Harvard-Smithsonian Center for Astrophysics, Cambridge, MA 02138, USA*
[2] *Quantum Technology Center, University of Maryland, College Park, MD 20742, USA*
[3] *Department of Physics, University of Maryland, College Park, MD 20742, USA*
[4] *Department of Electrical and Computer Engineering, University of Maryland, College Park, MD 20742, USA*

(Dated: April 15, 2021)

## SPIN PERIOD ANALYSIS

### Preparing the Data

After selecting our pulsars, we compute $f$ and $a$ for each pulsar from $P, \dot{P}, \mu, D, l, b$. The catalogue also supplies uncertainties $\sigma_P, \sigma_{\dot{P}}, \sigma_\mu$. For distance uncertainties, we use the following prescription:

$$\sigma_D = \begin{cases} \left.\begin{array}{l} \sigma_{D_\mathrm{A}} \text{ if it exists OR} \\ \max\left(D_\mathrm{A}^\mathrm{max} - D_\mathrm{A}, D_\mathrm{A} - D_\mathrm{A}^\mathrm{min}\right) \end{array}\right\} & \text{for } D = D_\mathrm{A}, \\ \sigma_\varpi / \varpi^2, & \text{if } D = 1/\varpi, \\ 0.4\, D_\mathrm{DM}, & \text{if } D = D_\mathrm{DM}. \end{cases}$$

The distance $D_\mathrm{A}$ is a distance obtained from association with another object or using some other reliable independent measurement. This type of distance measurement may come with an uncertainty $\sigma_{D_\mathrm{A}}$ or bounds $D_\mathrm{A}^\mathrm{min}, D_\mathrm{A}^\mathrm{max}$. If the distance is instead derived from a parallax measurement $\varpi$, we can estimate the distance error from the parallax uncertainty $\sigma_\varpi$. If no independent measurements exist, $D$ defaults to a model-based distance $D_\mathrm{DM}$ using the dispersion measure (DM) [1]. In this case, we adopt a conservative relative distance error of 40% in accordance with the RMS deviation in the `YMW16` model benchmarking results [2]. Lastly, we neglect uncertainties in right ascension and declination (which translate to errors in $l, b$) as they are negligible compared to other sources of error.

The covariance matrix for each observation is given by

$$\mathbf{\Sigma} = \begin{pmatrix} \sigma_f^2 & \sigma_{fa} \\ \sigma_{fa} & \sigma_a^2 \end{pmatrix}.$$

This matrix is estimated for each pulsar via (i) generating $f, a$ samples by drawing from all the constituent independent distributions (i.e., $\mathcal{N}(P, \sigma_P^2)$, $\mathcal{N}(\dot{P}, \sigma_{\dot{P}}^2)$, $\mathcal{N}(\mu, \sigma_\mu^2)$ and $\mathcal{N}(D, \sigma_D^2)$, all assumed to be normally distributed) and (ii) numerically computing the covariance of the samples. We are aware that the true joint $f, a$-distribution for each point may well be non-Gaussian in nature (esp. for pulsars with parallax-derived distances), but this consideration is beyond the scope of our analysis.

### Fitting the Data

For each pulsar in our dataset (labelled $i$), we have knowledge of the quantities $f_i$, $\sigma_{fi}$, $a_i$ and $\sigma_{ai}$. These are the $f$-coordinate, $f$-uncertainty, acceleration and acceleration uncertainty respectively for the $i^\mathrm{th}$ pulsar. Since $f$ and $a$ are not independent (both depend on $D$), we also need to take into account the covariance $\sigma_{fa}$. To simultaneously fit the local acceleration $a_0$ and the braking distribution $a_\mathrm{br}$ in the presence of statistical outliers, we use a Bayesian mixture model [3]. The mixture model has two components – a foreground distribution with the parameters of interest (i.e., slope $a_0$, braking parameter $\lambda$) and a broad background distribution representing the outliers. The background is parametrized by three nuisance parameters $P_\mathrm{bg}$, $\mu_\mathrm{bg}$ and $V_\mathrm{bg}$, which correspond to the relative amplitude, mean and variance of the background distribution respectively. Loosely speaking, $P_\mathrm{bg}$ can be thought of as the probability that a point is bad. Our likelihood function $\mathcal{L} \equiv \Pr\left(\{a_i\} | a_0, \lambda, P_\mathrm{bg}, \mu_\mathrm{bg}, V_\mathrm{bg}\right)$ is given by the expression

$$\mathcal{L} \propto \prod_i \left[ (1 - P_\mathrm{bg})\, \varphi_\mathcal{N}\left(\frac{a_i - a_0 f_i}{\sqrt{V_i}}\right) * \varphi_\mathcal{R}\left(\frac{a_i}{\lambda}\right) + P_\mathrm{bg} \varphi_\mathcal{N}\left(\frac{a_i - \mu_\mathrm{bg}}{\sqrt{\sigma_{ai}^2 + V_\mathrm{bg}}}\right)\right], \tag{1}$$

---

*,† These authors contributed equally to this work.

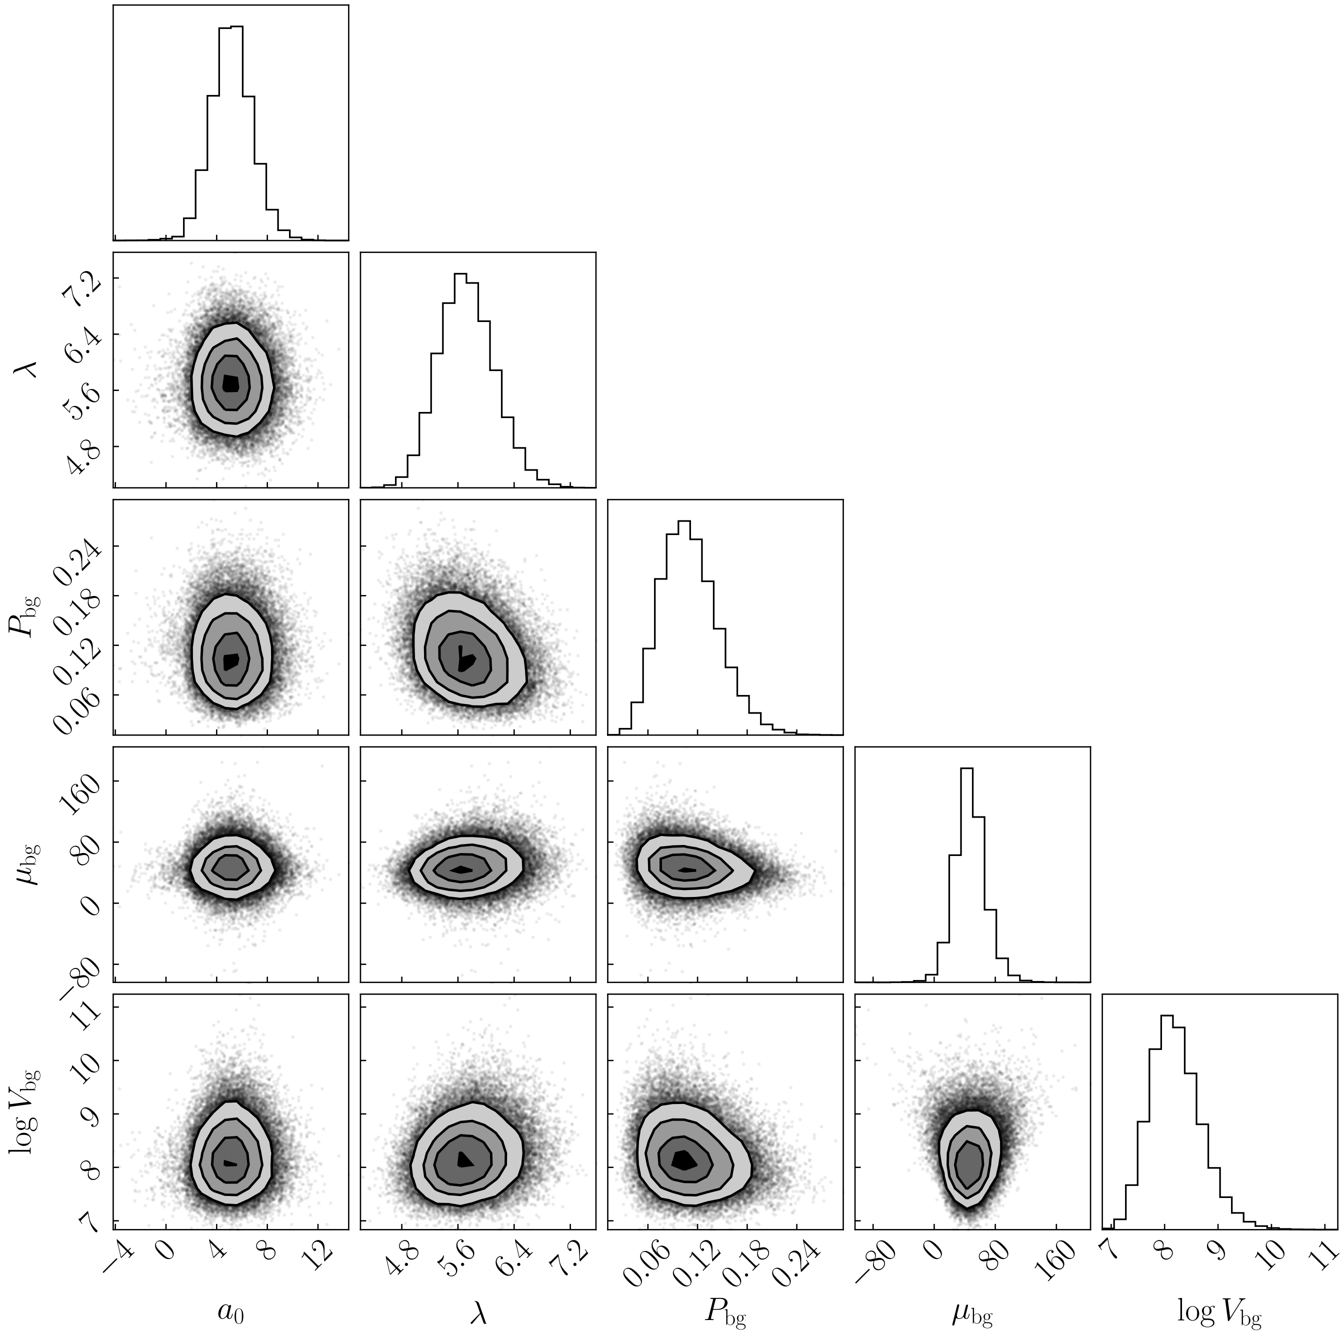


Figure 1. Corner plot visualizing samples drawn from the posterior distribution.

where the weight for each observation in the first term is then related to the variance $V_i = \sigma_{ai}^2 + a_0^2\sigma_{fi}^2 - 2a_0\sigma_{fai}$. The function $\varphi_{\mathcal{N}}(x) = \exp\left(-x^2/2\right)/\sqrt{2\pi}$ is the standard normal distribution. Similarly, $\varphi_{\mathcal{R}}(x) = x\exp\left(-x^2/2\right)$ is the standard Rayleigh distribution. Finally, the symbol $*$ denotes a convolution.

We choose uninformative priors for our parameters: $a_0 \sim \mathcal{U}(-20, 20)$, $\lambda \sim \mathcal{U}(0, 10)$, $P_{\rm bg} \sim \mathcal{U}(0, 1)$, $\mu_{\rm bg} \sim \mathcal{U}(-500, 500)$ and $\log_{\rm e} V_{\rm bg} \sim \mathcal{U}(2, 16)$. The quantities $a_0, \lambda, \mu_{\rm bg}, \sqrt{V_{\rm bg}}$ are all accelerations, which are expressed in units of $10^{-10}\mathrm{m/s^2}$, while $P_{\rm bg}$ is dimensionless. Multiplying this box prior with the likelihood defined earlier gives us the posterior distribution for our analysis. Parameter estimation is then a matter of sampling the posterior and finding the maximum — we do this with a Markov Chain Monte Carlo (MCMC) sampler [4]. The maximum a posteriori estimate is taken to be the best-fit estimate and samples drawn from the joint $a_0, \lambda$ posterior distribution are taken to represent the distribution of fitted accelerations. The samples are shown in Figure 1. Negligible correlations are observed between parameters.

The probability of any given point being "bad" (i.e., favoring the background distribution over the foreground distri-

bution) is given by

$$P_i^{\rm out} = \left\langle \frac{P_{\rm bg}\varphi_{\mathcal{N}}\left(\frac{a_i-\mu_{\rm bg}}{\sqrt{\sigma_{ai}^2+V_{\rm bg}}}\right)}{(1-P_{\rm bg})\,\varphi_{\mathcal{N}}\left(\frac{a_i-a_0 f_i}{\sqrt{V_i}}\right) * \varphi_{\mathcal{R}}\left(\frac{a_i}{\lambda}\right) + P_{\rm bg}\varphi_{\mathcal{N}}\left(\frac{a_i-\mu_{\rm bg}}{\sqrt{\sigma_{ai}^2+V_{\rm bg}}}\right)} \right\rangle, \tag{2}$$

where $\langle \ldots \rangle$ denotes an average over all MCMC samples. We call this the *outlier score*, and it takes on values between 0 and 1. The score represents the degree of certainty with which a point is classified as an outlier. Outlier scores for each of the 117 pulsars are given in Table I.

As mentioned in the main text, the mixture model discards about 10% of the pulsars in practice. To see if there was any systematic correlation with the type of distance estimates used for the pulsars (i.e., the largest source of error), we divided our set of 117 pulsars into two subsets — (1) pulsars with association-derived and parallax-derived distances (44 pulsars) and (2) pulsars with DM-derived distances (73 pulsars). We then re-ran the analysis on the subsets. Approximately 9% of the pulsars in subset 1 were discarded and approximately 15% of the the pulsars in subset 2 were discarded. Therefore, no dramatic difference is seen in the quality of data between the two subsets. However, the DM-derived distances are crucial to achieving a good acceleration sensitivity because distant pulsars (i.e., nonzero $f$) usually have DM-derived distances.

## Outlier Scores and Uncertainties in Spin Period Analysis

Table I below lists the outlier scores and the fractional contributions to acceleration uncertainties from both timing parameters (i.e., period and period derivative) and geometric parameters (i.e., distance and proper motion) for each of the 117 pulsars used in the spin period analysis. Outlier scores, $P^{\rm out}$, are described above in Eq. (2) and represent the likelihood that a pulsar is a member of the background distribution rather than a pulsar used to determine the acceleration. The table also provides two fractional uncertainties: $\sigma_{c\dot{P}/P}/\sigma_a$ is the fraction of the uncertainty in the acceleration associated with the term $c\dot{P}/P$ (derived from timing measurements) and $\sigma_{\mu^2 D}/\sigma_a$ is the fraction associated with the term $\mu^2 D$ (derived from proper motion and distance measurements). Finally, $\sigma_a$ is the total uncertainty in the acceleration. Note that the fractional contributions sum in quadrature to unity.

Table I: Outlier scores, $P^{\rm out}$, and fractional uncertainty contributions from timing parameters, $\sigma_{c\dot{P}/P}/\sigma_a$, and proper motion/distance, $\sigma_{\mu^2 D}/\sigma_a$, along with the total acceleration uncertainty $\sigma_a$ in units of $10^{-10}$ m/s$^2$ for 117 pulsars used in spin period analysis. See Eq. (2) for details on outlier scores. Higher outlier scores favor the background distribution.

| Pulsar | $P^{\rm out}$ | $\sigma_{c\dot{P}/P}/\sigma_a$ | $\sigma_{\mu^2 D}/\sigma_a$ | $\sigma_a$ | Pulsar | $P^{\rm out}$ | $\sigma_{c\dot{P}/P}/\sigma_a$ | $\sigma_{\mu^2 D}/\sigma_a$ | $\sigma_a$ |
|---|---|---|---|---|---|---|---|---|---|
| J1811-2405 | 1.000 | 0.00 | 1.00 | 0.27 | J1804-2717 | 0.011 | 0.01 | 1.00 | 1.70 |
| J1905+0400 | 1.000 | 0.46 | 0.88 | 0.00 | J0824+0028 | 0.011 | 0.01 | 1.00 | 5.35 |
| J0636+5129 | 1.000 | 0.00 | 1.00 | 0.55 | J1903-7051 | 0.011 | 0.00 | 1.00 | 0.12 |
| J0610-2100 | 1.000 | 0.01 | 1.00 | 1.07 | J1923+2515 | 0.010 | 0.00 | 1.00 | 0.71 |
| J0437-4715 | 1.000 | 0.01 | 1.00 | 0.61 | J0711-6830 | 0.010 | 0.02 | 1.00 | 4.79 |
| J1600-3053 | 1.000 | 0.02 | 1.00 | 0.60 | J1903+0327 | 0.010 | 0.01 | 1.00 | 0.09 |
| J1843-1113 | 1.000 | 0.00 | 1.00 | 4.17 | J1955+2527 | 0.010 | 0.00 | 1.00 | 2.88 |
| J1640+2224 | 0.944 | 0.00 | 1.00 | 0.57 | J1421-4409 | 0.010 | 0.06 | 1.00 | 0.26 |
| J1035-6720 | 0.719 | 0.08 | 1.00 | 0.22 | J1713+0747 | 0.009 | 0.00 | 1.00 | 0.28 |
| J2234+0611 | 0.716 | 0.00 | 1.00 | 0.54 | J1959+2048 | 0.009 | 0.01 | 1.00 | 1.05 |
| J1400-1431 | 0.267 | 0.00 | 1.00 | 1.58 | J1843-1448 | 0.009 | 0.00 | 1.00 | 2.34 |
| J1909-3744 | 0.246 | 0.00 | 1.00 | 4.69 | J1231-1411 | 0.009 | 0.01 | 1.00 | 0.51 |
| J1813-2621 | 0.222 | 0.15 | 0.99 | 0.06 | J0154+1833 | 0.009 | 0.07 | 1.00 | 0.12 |
| J2234+0944 | 0.164 | 0.00 | 1.00 | 1.23 | J2241-5236 | 0.009 | 0.00 | 1.00 | 0.26 |
| J1730-2304 | 0.159 | 0.00 | 1.00 | 0.36 | J1453+1902 | 0.009 | 0.06 | 1.00 | 0.41 |
| J0751+1807 | 0.111 | 0.00 | 1.00 | 2109.96 | J1709+2313 | 0.009 | 0.04 | 1.00 | 0.87 |
| J1944+0907 | 0.111 | 1.00 | 0.05 | 0.66 | J0509+0856 | 0.009 | 0.02 | 1.00 | 0.28 |
| J0645+5158 | 0.101 | 0.00 | 1.00 | 266.04 | J1801-3210 | 0.009 | 0.00 | 1.00 | 0.11 |
| J2033+1734 | 0.092 | 0.02 | 1.00 | 1.90 | J1012+5307 | 0.009 | 0.06 | 1.00 | 3.12 |
| J1142+0119 | 0.076 | 0.01 | 1.00 | 14.31 | J1955+6708 | 0.008 | 0.00 | 1.00 | 0.52 |
| J1024-0719 | 0.071 | 0.00 | 1.00 | 54.37 | J1721-2457 | 0.008 | 0.00 | 1.00 | 1.42 |
| J1455-3330 | 0.069 | 0.00 | 1.00 | 12.28 | J1719-1438 | 0.008 | 0.00 | 1.00 | 2.55 |
| J2339-0533 | 0.051 | 0.01 | 1.00 | 0.17 | J1732-5049 | 0.008 | 0.03 | 1.00 | 0.02 |
| J2010-1323 | 0.050 | 0.81 | 0.59 | 2.51 | J1939+2134 | 0.008 | 0.00 | 1.00 | 0.33 |
| J1902-5105 | 0.050 | 0.20 | 0.98 | 0.06 | J2042+0246 | 0.008 | 0.00 | 1.00 | 0.13 |
| J1630+3734 | 0.042 | 0.01 | 1.00 | 0.33 | J0740+6620 | 0.008 | 0.00 | 1.00 | 2.77 |

| | | | | |
|---|---|---|---|---|
| J1125+7819 | 0.038 | 0.01 | 1.00 | 6.52 |
| J1431-4715 | 0.038 | 0.03 | 1.00 | 0.27 |
| J2017+0603 | 0.038 | 0.00 | 1.00 | 23.87 |
| J1552-4937 | 0.036 | 0.00 | 1.00 | 19.25 |
| J1946+3417 | 0.034 | 0.00 | 1.00 | 0.11 |
| J1918-0642 | 0.034 | 0.02 | 1.00 | 0.28 |
| J0614-3329 | 0.029 | 0.01 | 1.00 | 2.11 |
| J1614-2230 | 0.029 | 0.00 | 1.00 | 11.97 |
| J1227-4853 | 0.027 | 0.07 | 1.00 | 0.06 |
| J1017-7156 | 0.026 | 0.03 | 1.00 | 0.09 |
| J1337-6423 | 0.024 | 0.00 | 1.00 | 9.88 |
| J1300+1240 | 0.023 | 0.04 | 1.00 | 0.74 |
| J1911-1114 | 0.022 | 0.00 | 1.00 | 0.96 |
| J1543-5149 | 0.020 | 0.00 | 1.00 | 1.62 |
| J0931-1902 | 0.018 | 0.03 | 1.00 | 5.82 |
| J2019+2425 | 0.018 | 0.00 | 1.00 | 3.65 |
| J2051-0827 | 0.018 | 0.00 | 1.00 | 0.59 |
| J1312+0051 | 0.017 | 0.00 | 1.00 | 6.70 |
| J0218+4232 | 0.016 | 0.01 | 1.00 | 3.44 |
| J1911+1347 | 0.016 | 0.00 | 1.00 | 1.95 |
| J0034-0534 | 0.016 | 0.01 | 1.00 | 1.01 |
| J1853+1303 | 0.015 | 0.01 | 1.00 | 0.05 |
| J2229+2643 | 0.014 | 0.00 | 1.00 | 0.33 |
| J1708-3506 | 0.014 | 0.01 | 1.00 | 0.08 |
| J1738+0333 | 0.014 | 0.00 | 1.00 | 1.74 |
| J2322-2650 | 0.013 | 0.00 | 1.00 | 5.05 |
| J1514-4946 | 0.013 | 0.02 | 1.00 | 0.96 |
| J1731-1847 | 0.012 | 0.01 | 1.00 | 2.41 |
| J2302+4442 | 0.012 | 0.00 | 1.00 | 0.14 |
| J1045-4509 | 0.012 | 0.00 | 1.00 | 5.75 |
| J1723-2837 | 0.011 | 0.15 | 0.99 | 0.38 |
| J1747-4036 | 0.011 | 0.03 | 1.00 | 0.21 |
| J2317+1439 | 0.006 | 0.00 | 1.00 | 0.64 |
| J1801-1417 | 0.008 | 0.47 | 0.89 | 0.10 |
| J1643-1224 | 0.008 | 0.01 | 1.00 | 0.22 |
| J1745+1017 | 0.007 | 0.03 | 1.00 | 0.16 |
| J1125-5825 | 0.007 | 0.06 | 1.00 | 1.39 |
| J1910+1256 | 0.007 | 0.00 | 1.00 | 1.77 |
| J0340+4130 | 0.007 | 0.00 | 1.00 | 0.14 |
| J0337+1715 | 0.007 | 0.36 | 0.94 | 0.01 |
| J2129-5721 | 0.007 | 0.41 | 0.91 | 1.64 |
| J1327-0755 | 0.007 | 0.02 | 1.00 | 0.18 |
| J1744-1134 | 0.007 | 0.04 | 1.00 | 0.90 |
| J1446-4701 | 0.007 | 0.09 | 0.99 | 0.25 |
| J2322+2057 | 0.007 | 0.00 | 1.00 | 1.80 |
| J1816+4510 | 0.007 | 0.00 | 1.00 | 0.04 |
| J0613-0200 | 0.007 | 0.03 | 1.00 | 0.06 |
| J1751-2857 | 0.007 | 0.08 | 1.00 | 0.87 |
| J2214+3000 | 0.007 | 0.00 | 1.00 | 1.00 |
| J0030+0451 | 0.007 | 0.04 | 1.00 | 0.83 |
| J2043+1711 | 0.007 | 0.00 | 1.00 | 0.38 |
| J1641+8049 | 0.007 | 0.04 | 1.00 | 1.05 |
| J1405-4656 | 0.007 | 0.00 | 1.00 | 0.54 |
| J0023+0923 | 0.007 | 0.00 | 1.00 | 0.59 |
| J1832-0836 | 0.007 | 0.00 | 1.00 | 1.07 |
| J1023+0038 | 0.006 | 0.02 | 1.00 | 0.60 |
| J1622-0315 | 0.006 | 0.01 | 1.00 | 0.04 |
| J1741+1351 | 0.006 | 0.01 | 1.00 | 0.68 |
| J1933-6211 | 0.006 | 0.02 | 1.00 | 0.04 |
| J2124-3358 | 0.006 | 0.00 | 1.00 | 0.11 |
| J1710+4923 | 0.006 | 0.00 | 1.00 | 0.88 |
| J0101-6422 | 0.006 | 0.02 | 1.00 | 0.06 |
| J1857+0943 | 0.006 | 0.00 | 1.00 | 0.04 |
| J1955+2908 | 0.006 | 0.00 | 1.00 | 0.24 |
| J1658-5324 | 0.006 | 0.00 | 1.00 | 0.21 |

## Monte Carlo Simulation

First, we approximate the $x$-, $y$- and $z$-distributions of pulsar locations in the current spin period dataset as normal distributions. Next, we draw $N$ locations (i.e., $(x, y, z)$ coordinates) from these distributions. From this set of locations, we can compute $f$ for each pulsar. The acceleration $a$ for each pulsar is given by a sum of $a_0^{\rm inj} f + a_{\rm br}$, where $a_0^{\rm inj} = 1.9 \times 10^{-10} {\rm m/s}^2$ is an injected acceleration, and $a_{\rm br}$ is a value drawn from the fitted braking distribution. The resulting data are fitted to a line and the standard deviation of the fitted slopes over 100 Monte Carlo runs is taken to be the local acceleration uncertainty $\sigma_{a_0}$ for a given $N$. The result as a function of $N$ is shown in Figure 2, averaging down as $N^{-1/2}$ as expected.

Our simulation neglects observational uncertainties in pulsar distances and proper motions. Thus, the number of pulsars required to reach a given sensitivity is to be taken as an order-of-magnitude estimate only.

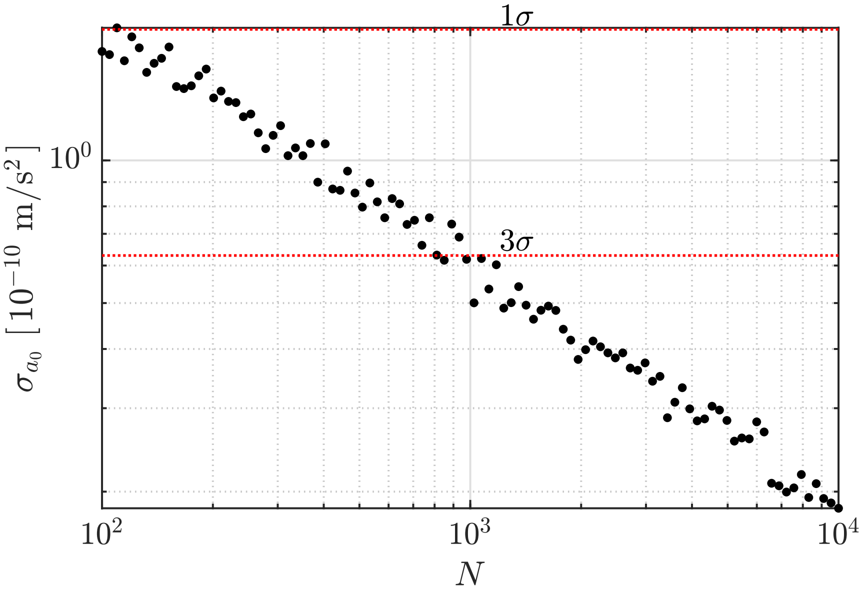


Figure 2. Monte Carlo simulation for acceleration sensitivity $\sigma_{a_0}$ vs. number of pulsars $N$ using spin period analysis. Statistical significance is given by comparing $\sigma_{a_0}$ to the nominally expected value of $a_0^{\rm inj} = 1.9 \times 10^{-10}{\rm m/s^2}$.

## ORBITAL PERIOD ANALYSIS

### Preparing the Data

Shao *et al.* [5] have provided a collection of pulsars in binary systems that have masses of both constituents measured. We used their sample as a starting point and retrieved all relevant parameters for our analysis from literature. Table II shows the data and uncertainties in measured parameters used for the orbital period analysis.

The orbital period decay due to gravitational wave emission is given by [6]

$$\dot{P}_{\rm b}^{\rm GW} = -\frac{192\pi}{5c^5}\eta(GM)^{5/3}n_{\rm b}^{5/3}\left(1+\frac{73}{24}e^2+\frac{37}{96}e^4\right)\left(1-e^2\right)^{-7/2}, \tag{3}$$

where $n_{\rm b} = 2\pi/P_{\rm b}$, $M \equiv M_1 + M_2$, and $\eta \equiv M_1M_2/M^2$. $G$, $c$, and $e$ are gravitational constant, speed of light, and orbital eccentricity, respectively. The observed acceleration has a contribution from this effect as $a_{\rm GW} = c\,\dot{P}_{\rm b}^{\rm GW}/P_{\rm b}$.

Observational covariance matrices were estimated by sampling as we did for spin periods, but this time sampling from $\mathcal{N}(P_{\rm b}, \sigma_{P_{\rm b}}^2)$, $\mathcal{N}(\dot{P}_{\rm b}, \sigma_{\dot{P}_{\rm b}}^2)$, $\mathcal{N}(\mu, \sigma_\mu^2)$, $\mathcal{N}(D, \sigma_D^2)$, $\mathcal{N}(M_1, \sigma_{M_1}^2)$, $\mathcal{N}(M_2, \sigma_{M_2}^2)$ and $\mathcal{N}(e, \sigma_e^2)$.

### Fitting the Data

In the orbital period analysis, the absence of a braking component greatly simplifies the model. Furthermore, the lack of statistical outliers allows us to forego the mixture model and adopt a very simple likelihood of the form

$$\mathcal{L} \propto \prod_i \varphi_{\mathcal{N}}\left(\frac{a_i - a_0 f_i}{\sqrt{V_i + V_{\rm int}}}\right), \tag{4}$$

where, $V_i = \sigma_{ai}^2 + a_0^2\sigma_{fi}^2 - 2a_0\sigma_{fai}$ as before, and $V_{\rm int}$ is a parameter representing intrinsic variance. We include this (nuisance) parameter because the intrinsic scatter in the $a_{\rm b}$ vs. $f$ data is not fully accounted for by $V_i$. In other words, not including $V_{\rm int}$ would underestimate the error bar on $a_0$.

We choose uninformative priors on our parameters: $a_0 \sim \mathcal{U}(-20, 20)$ and $\log_{\rm e} V_{\rm int} \sim \mathcal{U}(-5, 5)$. The quantities $a_0$ and $\sqrt{V_{\rm int}}$ are accelerations, which are expressed in units of $10^{-10}{\rm m/s^2}$. Once again, multiplying this box prior with the likelihood defined above gives us the posterior distribution. And as before, we sample the posterior and find its maximum using a MCMC sampler. The maximum a posteriori estimate is taken to be the best-fit estimate and samples drawn from the $a_0$ posterior distribution are taken to represent the distribution of fitted accelerations. The samples are shown in Figure 3; negligible correlations are observed between parameters.

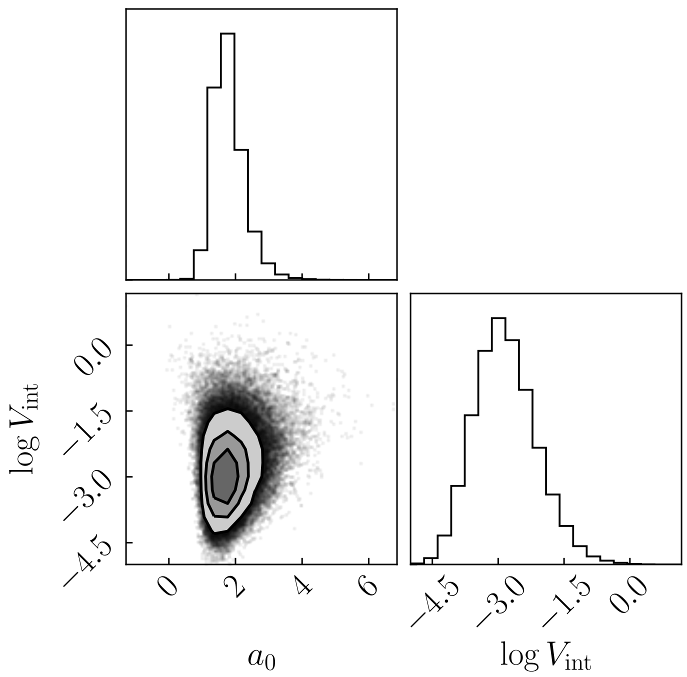


Figure 3. Corner plot visualizing samples drawn from the posterior distribution for orbital period analysis.

Table II: Binary pulsars used in orbital period analysis. For each pulsar, the first nine rows give relevant pulsar data for the calculation of accelerations and the last four rows give fractional acceleration uncertainty contributions from timing, $\sigma_{c\dot{P}_b/P_b}/\sigma_a$, gravitational wave emission, $\sigma_{c\dot{P}_b^{\rm GW}/P_b}/\sigma_a$, and astrometry/distances, $\sigma_{\mu^2 D}/\sigma_a$, along with the total acceleration uncertainty $\sigma_a$ in units of $10^{-10}$ m/s$^2$.

| Pulsar name | J0348+0432 [7] | J0437-4715 [8, 9] | J0613-0200 [9, 10] | J1012+5307 [9, 11] |
|---|---|---|---|---|
| Galactic longitude, $l$ [deg] | 183.3368 | 253.3943 | 210.413052 | 160.347 |
| Galactic latitude, $b$ [deg] | $-36.7736$ | $-41.963636$ | $-9.304907$ | 50.9858 |
| Distance, $D$ [kpc] | 2.1(2) | 0.15679(25) | 1.11(5) | 0.8(2) |
| Orbital period, $P_{\rm b}$ [days] | 0.102424062722(7) | 5.7410458(3) | 1.198512575184(13) | 0.604672723085(3) |
| Derivative of $P_{\rm b}$, $\dot{P}_{\rm b}$ [$10^{-12}$ s s$^{-1}$] | $-0.273(45)$ | 3.730(3) | 0.026(7) | 0.052(4) |
| Pulsar mass, $M_1$ [$M_\odot$] | 2.01(4) | 1.44(7) | 1.42(46) | 1.83(11) |
| Companion mass, $M_2$ [$M_\odot$] | 0.172(3) | 0.228(6) | 0.14(3) | 0.174(7) |
| Orbital eccentricity, $e$ [$10^{-6}$] | 2.6(9) | 19.182(1) | 4.50(9) | 1.1(1) |
| Total proper motion, $\mu$ [mas year$^{-1}$] | 5.3(4) | 140.852(1) | 10.514(17) | 25.737(18) |
| | | | | |
| $\sigma_{c\dot{P}_b/P_b}/\sigma_a$ | 0.99 | 0.45 | 0.97 | 0.23 |
| $\sigma_{c\dot{P}_b^{\rm GW}/P_b}/\sigma_a$ | 0.13 | 0.00 | 0.12 | 0.04 |
| $\sigma_{\mu^2 D}/\sigma_a$ | 0.00 | 0.90 | 0.19 | 0.97 |
| $\sigma_a$ [$10^{-10}$ ms$^{-2}$] | 15.23 | 0.04 | 0.21 | 0.99 |

| Pulsar name | J1022+1001 [9, 10] | B1534+12 [12] | J1713+0747 [9, 13] | J1738+0333 [14] |
|---|---|---|---|---|
| Galactic longitude, $l$ [deg] | 242.4 | 19.847526 | 28.750557 | 27.7213 |
| Galactic latitude, $b$ [deg] | 43.7 | 48.341431 | 25.222839 | 17.7422 |
| Distance, $D$ [kpc] | 0.72(2) | 1.051(5) | 1.20(3) | 1.47(10) |
| Orbital period, $P_{\rm b}$ [days] | 7.8051348(11) | 0.420737298879(2) | 67.825131000(1) | 0.3547907398724(13) |
| Derivative of $P_{\rm b}$, $\dot{P}_{\rm b}$ [$10^{-12}$ s s$^{-1}$] | 0.21(7) | $-0.1366(3)$ | 0.5(1) | $-0.0170(31)$ |
| Pulsar mass, $M_1$ [$M_\odot$] | 1.72(65) | 1.3330(2) | 1.33(10) | 1.46(06) |
| Companion mass, $M_2$ [$M_\odot$] | 1.03(36) | 1.3455(2) | 0.289(7) | 0.181(8) |
| Orbital eccentricity, $e$ [$10^{-6}$] | 97.04(5) | 273677.52(7) | 74.9402(4) | 0.34(11) |
| Total proper motion, $\mu$ [mas year$^{-1}$] | 18.4(89) | 25.328(11) | 6.289463(461) | 8.675(8) |
| | | | | |
| $\sigma_{c\dot{P}_b/P_b}/\sigma_a$ | 0.17 | 0.72 | 0.99 | 0.90 |
| $\sigma_{c\dot{P}_b^{\rm GW}/P_b}/\sigma_a$ | 0.00 | 0.08 | 0.00 | 0.41 |
| $\sigma_{\mu^2 D}/\sigma_a$ | 0.99 | 0.68 | 0.16 | 0.16 |
| $\sigma_a$ [$10^{-10}$ ms$^{-2}$] | 1.88 | 0.03 | 0.05 | 0.34 |

| Pulsar name | J1756-2251 [15] | J1909-3744 [9, 10] | B1913+16 [16, 17][a] | J2222-0137 [19] |
|---|---|---|---|---|
| Galactic longitude, $l$ [deg] | 6.498658 | 359.7 | 49.967651 | 62.0184 |
| Galactic latitude, $b$ [deg] | 0.94801 | $-19.6$ | 2.121891 | $-46.0753$ |
| Distance, $D$ [kpc] | 0.95(50) | 1.14(1) | 9(3) | 0.2673(10) |
| Orbital period, $P_{\rm b}$ [days] | 0.31963390143(3) | 1.533449475278(1) | 0.322997448918(3) | 2.44576456(13) |
| Derivative of $P_{\rm b}$, $\dot{P}_{\rm b}$ [$10^{-12}$ s s$^{-1}$] | $-0.229(5)$ | 0.503(5) | $-2.423(1)$ | 0.27(9) |
| Pulsar mass, $M_1$ [$M_\odot$] | 1.341(7) | 1.48(3) | 1.438(1) | 1.76(6) |
| Companion mass, $M_2$ [$M_\odot$] | 1.230(7) | 0.209(1) | 1.390(1) | 1.293(25) |
| Orbital eccentricity, $e$ ($10^{-6}$) | 180569.4(2) | 0.104(6) | 617134.0(4) | 38.0940(3) |
| Total proper motion, $\mu$ [mas year$^{-1}$] | 2.42$\pm$20[b] | 37.0197(88) | 1.483(55) | 45.09(2) |
| | | | | |
| $\sigma_{c\dot{P}_b/P_b}/\sigma_a$ | 0.27 | 0.76 | 0.43 | 1.00 |
| $\sigma_{c\dot{P}_b^{\rm GW}/P_b}/\sigma_a$ | 0.08 | 0.01 | 0.88 | 0.00 |
| $\sigma_{\mu^2 D}/\sigma_a$ | 0.96 | 0.66 | 0.20 | 0.01 |
| $\sigma_a$ [$10^{-10}$ ms$^{-2}$] | 2.00 | 0.15 | 0.25 | 1.27 |

[a] There is some disagreement in the literature regarding the distance and proper motion of B1913+16. We rely on the values from [17]. However, using results from [18] does not significantly change the acceleration extracted from this analysis.
[b] The proper motion in the right ascension direction ($\mu_\alpha$) is measured to be $-2.42(8)$ mas/yr. However, the proper motion in declination ($\mu_\delta$) is only bounded as $< 20$ mas/yr, so we assume $\mu_\delta = 0 \pm 20$ mas/yr.

| Pulsar name | J1829+2456 [20] |
|---|---|
| Galactic longitude, $l$ [deg] | 53.3424 |
| Galactic latitude, $b$ [deg] | 15.612 |
| Distance, $D$ [kpc] | 0.91(36) |
| Orbital period, $P_{\rm b}$ [days] | 1.17602795267(18) |
| Derivative of $P_{\rm b}$, $\dot{P}_{\rm b}$ [$10^{-12}$ s s$^{-1}$] | −0.05(2) |
| Pulsar mass, $M_1$ [$M_\odot$] | 1.295 (11) |
| Companion mass, $M_2$ [$M_\odot$] | 1.9(6) |
| Orbital eccentricity, $e$ [$10^{-6}$] | 139143.7(3) |
| Total proper motion, $\mu$ [mas year$^{-1}$] | 9.41(8) |
| | |
| $\sigma_{c\dot{P}_b/P_b}/\sigma_a$ | 0.87 |
| $\sigma_{c\dot{P}_b^{\rm GW}/P_b}/\sigma_a$ | 0.35 |
| $\sigma_{\mu^2 D}/\sigma_a$ | 0.34 |
| $\sigma_a$ [$10^{-10}$ ms$^{-2}$] | 0.68 |

* dphillips@cfa.harvard.edu
† aakash.ravi@gmail.com

[1] A. Lyne and F. Graham-Smith, *Pulsar Astronomy*, 4th ed. (Cambridge University Press, 2012).
[2] J. M. Yao, R. N. Manchester, and N. Wang, Astrophys. J. **835**, 29 (2017).
[3] D. W. Hogg, J. Bovy, and D. Lang, (2010), arXiv:1008.4686 [astro-ph.IM].
[4] D. Foreman-Mackey, D. W. Hogg, D. Lang, and J. Goodman, Publ. Astron. Soc. Pac. **125**, 306 (2013).
[5] L. Shao, N. Wex, and S.-Y. Zhou, Phys. Rev. D **102**, 024069 (2020).
[6] P. C. Peters and J. Mathews, Phys. Rev. **131**, 435 (1963).
[7] J. Antoniadis, P. C. Freire, N. Wex, T. M. Tauris, R. S. Lynch, M. H. van Kerkwijk, M. Kramer, C. Bassa, V. S. Dhillon, T. Driebe, *et al.*, Science **340**, 6131 (2013).
[8] D. Reardon, G. Hobbs, W. Coles, Y. Levin, M. Keith, M. Bailes, N. Bhat, S. Burke-Spolaor, S. Dai, M. Kerr, *et al.*, Mon. Not. Roy. Astron. Soc. **455**, 1751 (2016).
[9] B. Perera, M. DeCesar, P. Demorest, M. Kerr, L. Lentati, D. Nice, S. Osłowski, S. Ransom, M. Keith, Z. Arzoumanian, *et al.*, Mon. Not. Roy. Astron. Soc. **490**, 4666 (2019).
[10] G. Desvignes, R. Caballero, L. Lentati, J. Verbiest, D. Champion, B. Stappers, G. Janssen, P. Lazarus, S. Osłowski, S. Babak, *et al.*, Mon. Not. Roy. Astron. Soc. **458**, 3341 (2016).
[11] K. Lazaridis, N. Wex, A. Jessner, M. Kramer, B. Stappers, G. Janssen, G. Desvignes, M. Purver, I. Cognard, G. Theureau, *et al.*, Mon. Not. Roy. Astron. Soc. **400**, 805 (2009).
[12] E. Fonseca, I. H. Stairs, and S. E. Thorsett, Astrophys. J. **787**, 82 (2014).
[13] W. Zhu, G. Desvignes, N. Wex, R. Caballero, D. Champion, P. Demorest, J. Ellis, G. Janssen, M. Kramer, A. Krieger, *et al.*, Mon. Not. Roy. Astron. Soc. **482**, 3249 (2019).
[14] P. C. Freire, N. Wex, G. Esposito-Farese, J. P. Verbiest, M. Bailes, B. A. Jacoby, M. Kramer, I. H. Stairs, J. Antoniadis, and G. H. Janssen, Mon. Not. Roy. Astron. Soc. **423**, 3328 (2012).
[15] R. D. Ferdman, I. H. Stairs, M. Kramer, G. H. Janssen, C. G. Bassa, B. W. Stappers, P. B. Demorest, I. Cognard, G. Desvignes, G. Theureau, *et al.*, Mon. Not. Roy. Astron. Soc. **443**, 2183 (2014).
[16] J. M. Weisberg and Y. Huang, Astrophys. J. **829**, 55 (2016).
[17] J. M. Weisberg, S. Stanimirović, K. Xilouris, A. Hedden, A. de la Fuente, S. B. Anderson, and F. A. Jenet, Astrophys. J. **674**, 286 (2008).
[18] A. T. Deller, J. M. Weisberg, D. J. Nice, and S. Chatterjee, Astrophys. J. **862**, 139 (2018).
[19] I. Cognard, P. C. Freire, L. Guillemot, G. Theureau, T. M. Tauris, N. Wex, E. Graikou, M. Kramer, B. Stappers, A. G. Lyne, *et al.*, Astrophys. J. **844**, 128 (2017).
[20] H. T. Haniewicz, R. D. Ferdman, P. C. Freire, D. J. Champion, K. A. Bunting, D. R. Lorimer, and M. A. McLaughlin, (2020), arXiv:2007.07565 [astro-ph.SR].
